# Supplementary material for: Limited knowledge exchange across biological subfields in agent-based modelling: an LLM-assisted bibliometric analysis
Source: arXiv:2611.06596 source file (2026-11-04)
Supplement: Supplementary file 1 [file supplementary_material.tex]

\documentclass[11pt, a4paper, oneside]{article}
\usepackage{inputenc}
\usepackage[section]{placeins}

\usepackage[maxbibnames=10, backend=biber, autocite=superscript, natbib, backend=bibtex, bibstyle=authoryear, giveninits=true,
style=authoryear,maxcitenames=2]{biblatex}%style=authoryear,maxcitenames=2citestyle=numeric
\usepackage{comment}
\usepackage{algorithm}
\usepackage{algpseudocode}
\usepackage{paralist}
\usepackage{setspace}
\addbibresource{references.bib}
\usepackage{setspace}
\usepackage{graphicx}
\usepackage{graphics}
\usepackage{wrapfig}
\usepackage{amsmath}
\usepackage{tabularx}
\usepackage[dvipsnames]{xcolor}
\usepackage[margin=2cm]{geometry}
\geometry{left=2.5cm, top=2.2cm, bottom=2.2cm, right=2.5cm}
\usepackage{mathtools}
\usepackage{tcolorbox}
\usepackage{float}
\usepackage[normalem]{ulem}
\definecolor{arsenic}{rgb}{0.23, 0.27, 0.29}
\usepackage[font=small,skip=5pt]{caption}
\usepackage{titlesec}
\usepackage{arydshln}
\usepackage{soul}
\usepackage{subcaption}
\usepackage{adjustbox}
\usepackage{lineno}
\usepackage{setspace}
\usepackage{multirow}
\usepackage{multicol}
\usepackage{listings}
\usepackage{titling}
\usepackage{array}
\usepackage{makecell}
\usepackage{MnSymbol}
\usepackage{mathtools}
\usepackage{scrextend}
\usepackage{caption}
\usepackage{hyperref}
\usepackage{siunitx}
\DeclareSIUnit{\Molar}{\textsc{M}}
\DeclareCiteCommand{\citeyearpar}
    {}
    {\mkbibparens{\bibhyperref{\printdate}}}
    {\multicitedelim}
    {}
\renewcommand*{\bibfont}{\normalfont\small}
\captionsetup{font=small}
\usepackage{etoolbox}
\AtBeginEnvironment{tabular}{\small}

\renewcommand{\thesection}{SM\arabic{section}}  
\renewcommand{\thetable}{SM\arabic{table}}  
\renewcommand{\thefigure}{SM\arabic{figure}}

\makeatletter
\setlength{\@fptop}{0pt}
\makeatother

\begin{document}



\bigskip
{\Large
\noindent {\bf \emph{Supplementary material to}} Limited knowledge exchange across biological subfields in agent-based modelling: 
an LLM-assisted bibliometric analysis}
\begin{flushleft}
\bigskip 
Kira Pugh\textsuperscript{1$\circledast$}, 
Rebecca M Crossley\textsuperscript{2}, 
Sara Hamis\textsuperscript{1}.

\begin{comment}
\bigskip
\textbf{1} Department of Information Technology, Uppsala University, Uppsala, Sweden. 
\\
\textbf{2} \textcolor{red}{Mathematical Institute, University of Oxford, Oxford, United Kingdom.}
%\textbf{2} Department of Mathematics, University of California Los Angeles, CA, USA.
\\
\end{comment}

\end{flushleft}

\begin{comment}
\smallskip
\noindent{\bf Author ORCiDs}: 
\smallskip
\textbf{KP:} 0000-0001-5588-7014; 
\textbf{LG:} 0000-0002-8745-4480;
\textbf{SH:} 0000-0002-1105-8078.
\end{comment}

\bigskip
\noindent{\bf $\circledast$ Corresponding author}: kira.pugh@it.uu.se. 

\thispagestyle{empty} 

%
\newpage 
\clearpage
\pagenumbering{arabic} 

\section{Identifying previous bibliometric studies of ABMs}

To identify previous bibliometric analyses of ABM research, we conducted the following search in the WoS Core Collection (WoSCC):

\begin{tcolorbox}[
    colback=gray!10,
    colframe=gray!60,
    arc=1mm
    boxrule=1pt
]
\ttfamily
(TI=(bibliometric*) OR AB=(bibliometric*) OR AK=(bibliometric*))
%\\
AND
%\\
(TI=("agent-based model*" OR "individual-based model*")
%\\
OR AB=("agent-based model*" OR "individual-based model*")
%\\
OR AK=("agent-based model*" OR "individual-based model*"))
\end{tcolorbox}

\noindent This search query was conducted on 28 October 2026 and retrieved articles containing the term ``bibliometric*", together with ``agent-based model*" or ``individual-based model*" (or both) in the title (TI), abstract (AB), or author keywords (AK), identifying 47 articles published between 2011 and 2025.
%
Note that the asterisk denotes a wildcard that matches any word ending.


\vspace{0.5cm}


\section{Supporting information on citation patterns}

\vspace{0.5cm}

Figure \ref{fig:cross_talk_received} presents the reverse citation perspective of Figure 3b,c in the main manuscript, showing the proportion of citations \textit{received} from each subfield rather than those \textit{given} to each subfield.
%
Relative to subfield size, citations were concentrated within subfields: 86\%, 84\%, 69\%, and 57\% of citations received from ecology, epidemiology, oncology, and other-biology, respectively, went to articles in the same subfield (Figure~\ref{fig:cross_talk_received}a).
%
In the permutation test (Figure~\ref{fig:cross_talk_received}b), no permutation reached the observed values ($p \leq 0.001$ for all subfields).
%
The similarity between the two citation perspectives suggests that citation exchange between subfields is relatively reciprocal, rather than unidirectional.


\begin{figure}[h!]
    \centering
    \includegraphics[width=1\linewidth]{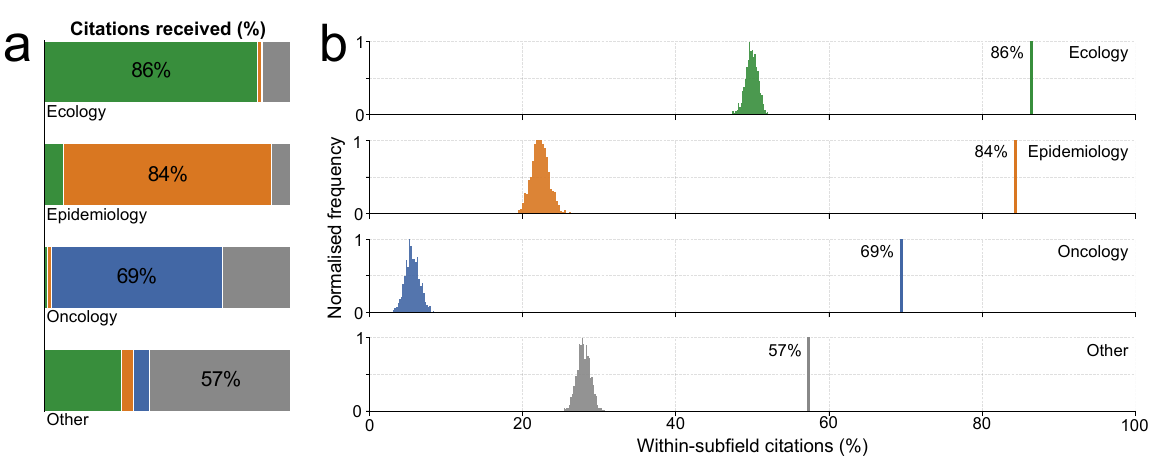}
    \caption{\textbf{Citation flows within and between biological subfields.}
    %
    Subfields are ecology, epidemiology, oncology, and the residual other-biology category, and only citations between articles in the biology dataset are included.
    %
    (a) Proportion of citations received from each citing subfield.
    %
    (b) Null distributions of within-subfield citation proportions from 1000 permutations, in which subfield labels were shuffled among articles within each publication year.
    %
    Vertical lines mark the observed values.}
    \label{fig:cross_talk_received}
\end{figure}



\newpage
\section{Supporting information on author overlap}

\subsection{Annual ORCID iD coverage}
Figure \ref{fig:orcid_over_time} shows a substantial increase in ORCID ID coverage across all four subfields between 1993 and 2025.
%
From 2010 onward, annual ORCID iD coverage exceeds 50\% in all four subfields. 
%
We therefore restrict the author overlap analysis in Section 3.3 to the period 2010--2025.
%

\vspace{0.5cm}

\begin{figure}[h!]
    \centering
    \includegraphics[width=1\linewidth]{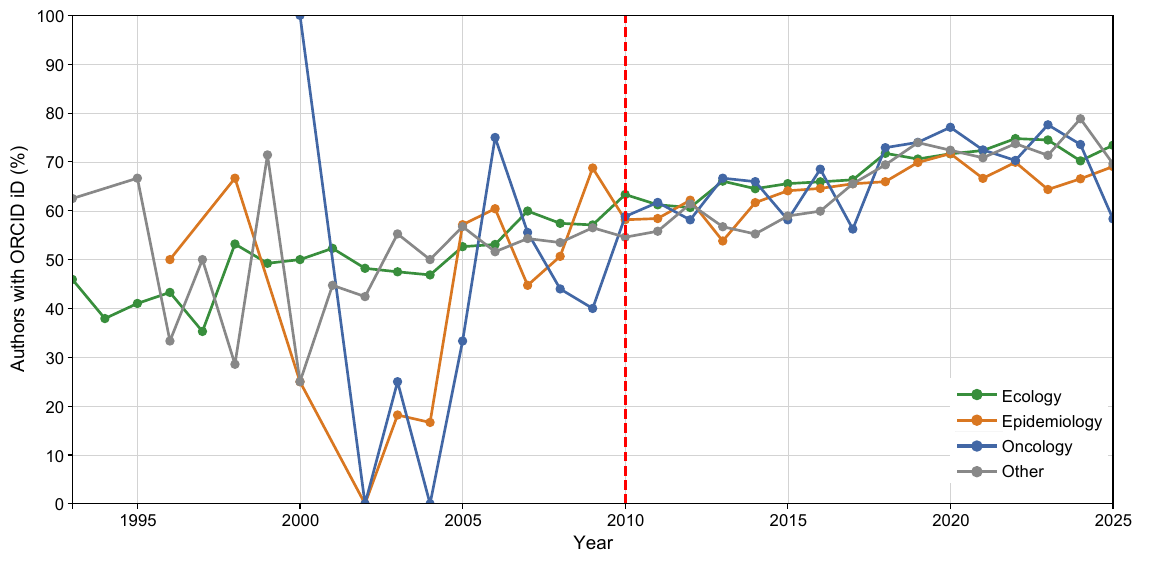}
    \caption{\textbf{Annual ORCID iD coverage across the four biological subfields.
    }
    %
    The red dashed vertical line indicates the first year from which annual ORCID iD coverage has since remained at least 50\% in all four subfields.
    }
    \label{fig:orcid_over_time}
\end{figure}


\vspace{0.5cm}

\subsection{Author overlap including other-biology}

We repeated the author overlap analysis described in Section 3.3 of the main manuscript, this time including the residual other-biology subfield in the analysis.
%
Out of the 2,954 authors, 72\% published in only one subfield (Figure~\ref{fig:orcid_venn}a,b), compared with 91\% when other-biology was excluded.
%
Including other-biology increased the proportion of authors publishing across multiple subfields to 34\%, 36\%, and 66\% for ecology, epidemiology, and oncology, respectively (Figure~\ref{fig:orcid_venn}c).
%
In the permutation test, overlap remained far below the null distribution for all subfields ($p \leq 0.001$).
%



\begin{figure}[t!]
\centering
    \includegraphics[width=1\linewidth]{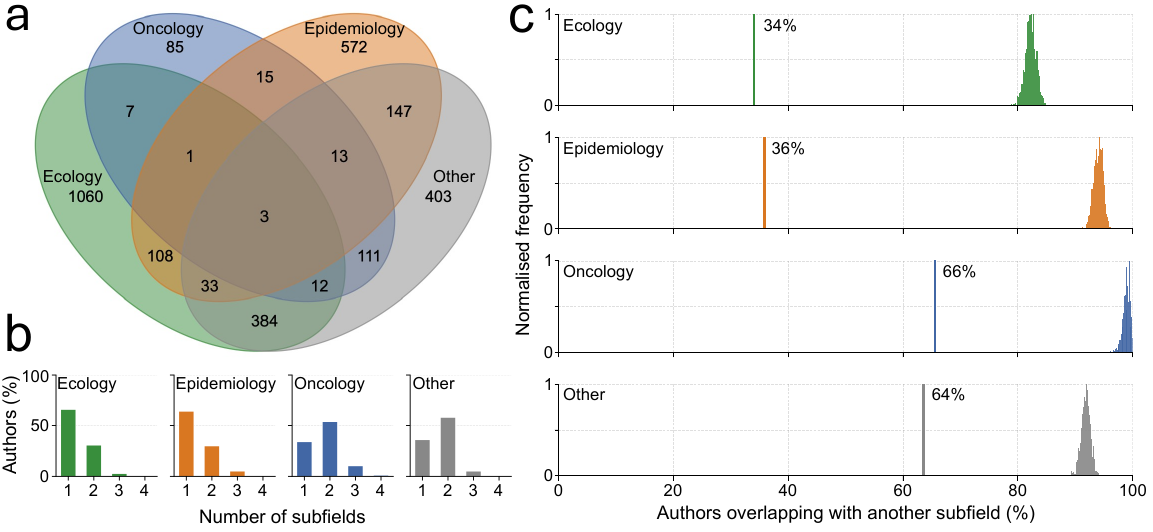}
    \caption{\textbf{Authors publishing within and across biological subfields.}
    %
    Subfields are ecology, epidemiology, oncology, and other-biology, and only authors with an ORCID iD and at least two articles across these subfields published between 2010 and 2025 are included.
    %
    (a) Number of unique authors publishing in each combination of subfields. 
    %
    (b) For authors who published in ecology, epidemiology, oncology, and other-biology (bars, left to right), the proportion who published in one, two, three, or four subfields. Colours as in (a). 
    %
    (c) Null distributions of author overlap from 1000 permutations, in which subfield labels were shuffled among the included articles within each publication year.
    %
    Vertical lines mark the observed values.
    }
    \label{fig:orcid_venn}

\end{figure}



\end{document}
